# Supplementary material for: High Pressure Suppression of Plasticity due to Over-Nucleation of Shear Strain
Source: arXiv:2402.08104 source file (2024-02-12)
Supplement: Supplementary file 1 [file Supplemental_Materials.pdf]

# Supplemental Materials to: High Pressure Suppression of Plasticity due to Over-Nucleation of Shear Strain

Brenden W. Hamilton and Timothy C. Germann

## SM-1: Extended Methods

All classical molecular dynamics (MD) simulations were performed using a fully flexible, non-polarizable force field from Smith and Bharadwaj. The model utilizes harmonic functions to describe bond stretch, angle bend, and dihedral and improper torsions. Non-bonded interactions are modeled using a Buckingham potential with an 11.0 A cutoff in which 1-3 binded pairs experience no interaction and 1-4 bonded pairs experience the full interaction. Electrostatics are solved for using the PPPM method.

A 1.0 fs timestep was used in all simulations. Shock simulation cells were constructed by replicating the alpha-RDX crystal structure along the [100], [010] and [001] directions, aligned with the x, y, and z Cartesian axis respectively, to lengths of 118.2nm, 34.3nm, and 31.8nm (30x10x10 unit cells), respectively. 5.0nm of material was removed, by whole molecules, at either end of the x-direction to break periodicity and form a free surface, which is necessary for the shock simulations. The system was then equilibrated for 500ps at 300 K using a Nose-Hoover thermostat, to allow breathing modes from the free surface creation to attenuate.

Shock simulations were conducted using the reverse ballistic approach along the [100] direction. The bottom 2.5nm in the x-direction, partitioned by whole molecules, was held rigid to form an infinitely massive piston. Particle velocities were initialized by adding the intended velocity to all non-piston molecules in addition to their thermal velocities. Particle velocities used were 0.7, 0.8, 0.9, 1.0, 1.1, and 1.2 km/s. When each shock reaches maximum compression, shock absorbing boundary conditions are applied to extend the simulation indefinitely. This is done by freezing the top 5.0 nm in the x-direction, partitioned by whole molecules, as a rigid system, with no velocities or forces at all time steps, equivalent to the initial piston. This holds the cell at the shock compression with no net-translation, representing a system in which the shock continues forward into an infinitely long sample. Shock release simulations were conducted by releasing this shock absorbing boundary at a later time, allowing the material to expand to alleviate the shock pressure.

All analysis done, including any binning, is done from a molecularly averaged framework. The per atom quantities of position, r, velocity, v, and stress, s, are summed in a center of mass framework

$$R = \frac{1}{M}\sum m_i r_i$$

$$V = \frac{1}{M} m_i v_i$$

$$S = \sum s_i$$

where M is the mass of an RDX molecule, m is the mass of atom i, and all sums are conducted over the 21 atoms of a molecule. All capital letters represent molecular values and lower case represent atomic values.

From these, we compute a total molecular kinetic energy and separate the contributions into a translational and roto-librational and vibrational kinetic energy:

$$KE_{Total} = \sum 0.5 m_i (v_i \cdot v_i)$$

$$KE_{Trans} = \frac{1}{2} M (V \cdot V)$$

$$KE_{ro-vib} = KE_{Total} - KE_{Trans}$$

The roto-librational and vibrational kinetic energy is then interpreted as the molecular temperature and is scaled to units of kelvin following the classical specific heat:

$$KE_{ro-vib} = \frac{3N-3}{2} k_B T$$

All molecular shear strains were calculated as the von Mises strain of the Green Lagrange strain tensor, as implemented in OVITO, using the unshocked system as the reference frame. Cluster analysis was conducted using the cluster tool in OVITO with a cutoff of 6.0 A, in which 5.0 A is the minimum value for which an un-defected single crystal is considered one cluster. Radial distribution functions were also calculated using the tool implemented in OVITO, as was the Wigner -Seitz defect analysis.

The $P_2[Cos(\theta)]$ metric is designed to show changes in rotational order. Theta is defined as the angle between two vectors Q, where Q is the vector normal to the plane formed by the 3 carbon atoms in the ring structure, such that

$$Cos(\theta) = Q(t) \cdot Q(0)$$

giving a rotational change in the molecular orientation with respect to the initial crystal structure. Using the second Legendre polynomial to normalize values, a value of 1 is no change in rotational order, and -0.5 is the maximum change. All values lower than 0.5 are considered greatly changed.

## SM-2: Shear Band Images

This section contains additional figures of the shear band network for the shocks conducted in this study. Figure S1 shows a slice of the X-Z plane of the material at maximum compression and 50ps held at maximum compression, the same as Figure 1 in the main manuscript, except the color bar of shear strain has been significantly widened to show the greater disparity.

Figure S2 shows results from shocks at 0.8 and 1.1 km/s with a 5x5 increase in size in the two cross section directions, showing that, compared to the smaller cell, no significant system size effects occur in the formation of the shear bands.

Figure S3 shows longer time history of the 1.2 km/s case in which the system is held at maximum compression for 450ps, in which no shear bands form and the shear of the system has little to no temporal evolution. Increased shear on the far left side of the images is due to continued friction with the piston.

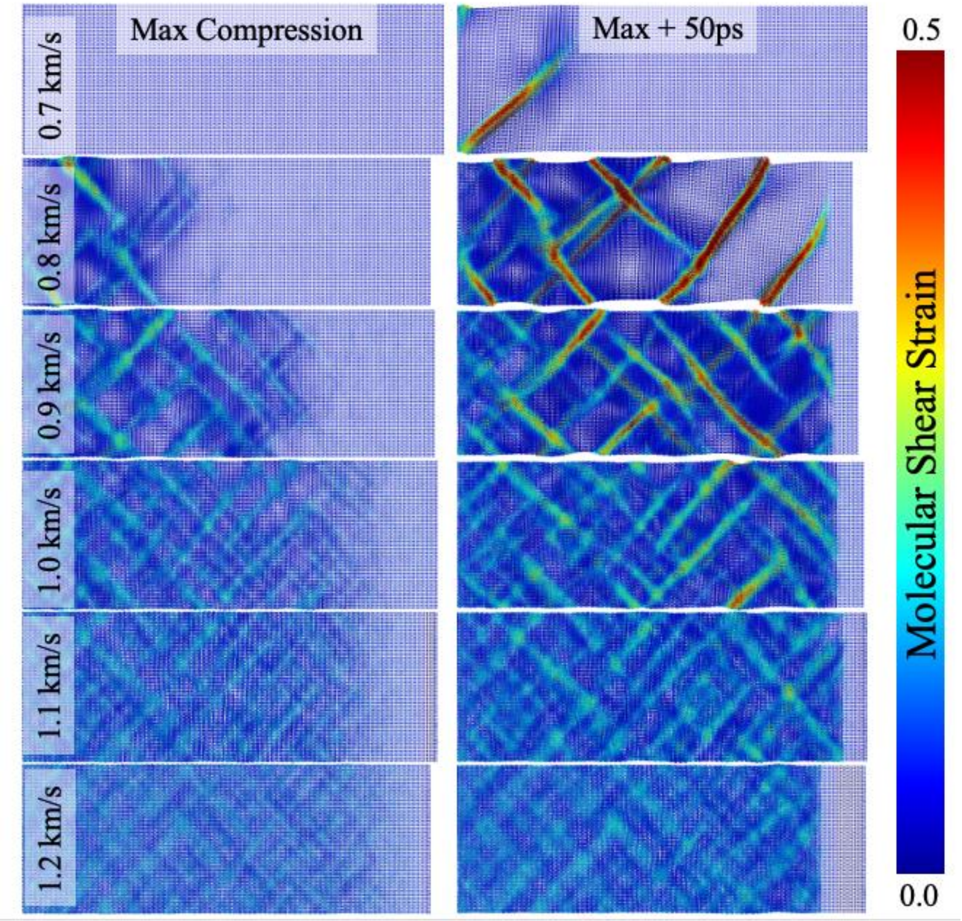


Figure S1: Molecular renderings of all shocks and max compression and max + 50ps, colored by shear strain.

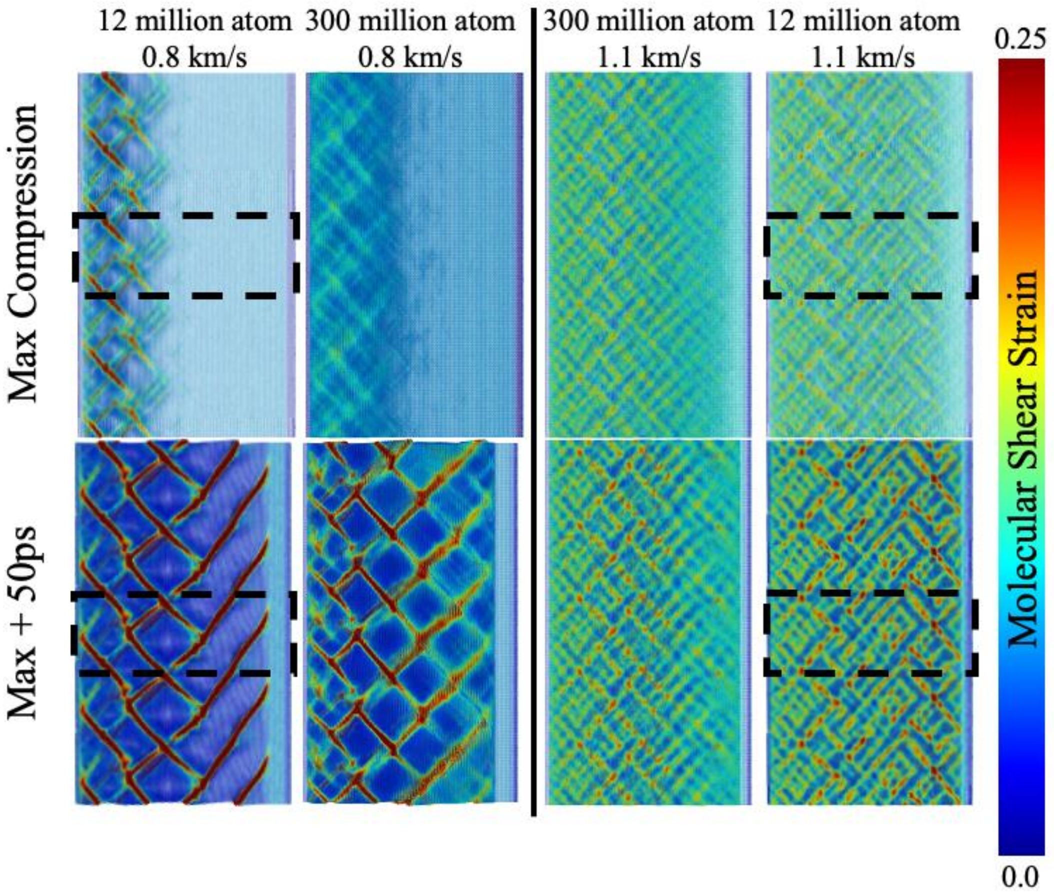


Figure S2: Shear strain colored molecular renderings for 12 and 300 million atom cells at 0.8 and 1.1 km/s for max compression and 50ps held at max compression.

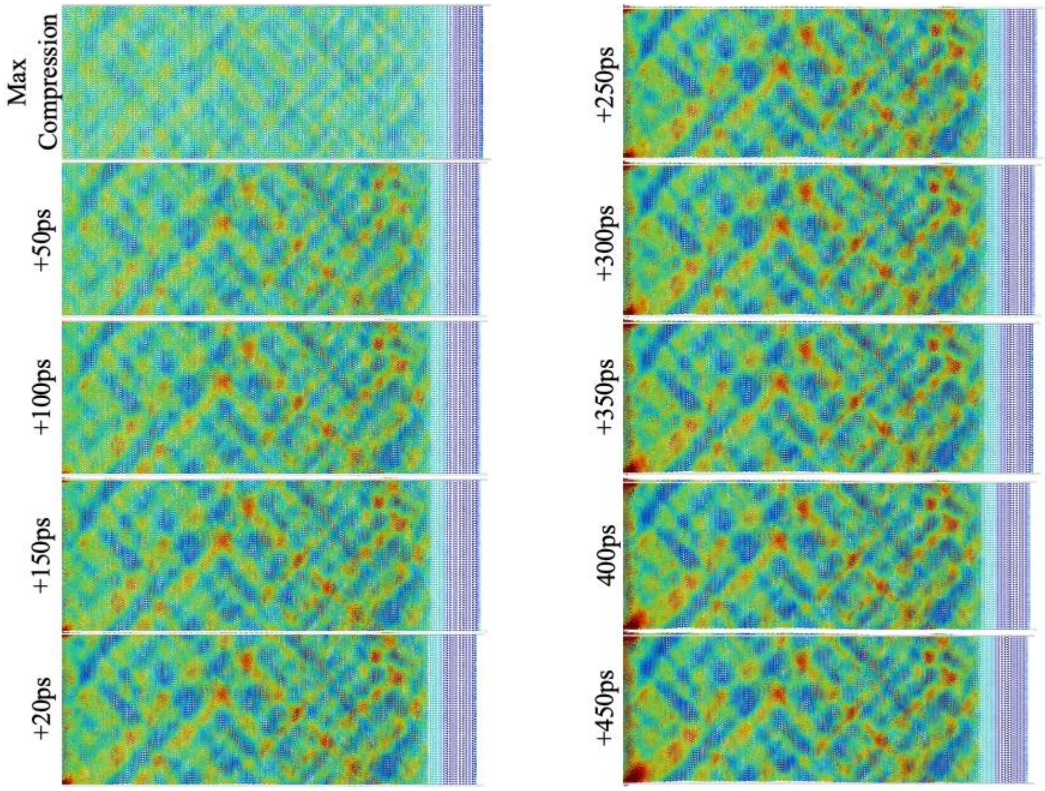


Figure S3: Additional molecular renderings of the 1.2 km/s case for being held at max compression for 450ps.

## SM-3: 1D Binned States

Figure S4 shows a 1D binning of the shear strains, showing that, despite the lack of shear bands, the stronger shocks result in slightly more shear strain per molecule or per volume than the shear banding cases due to the homogeneous nature of the shearing. Figure S5 shows the system wide distributions of these molecular shear strains.

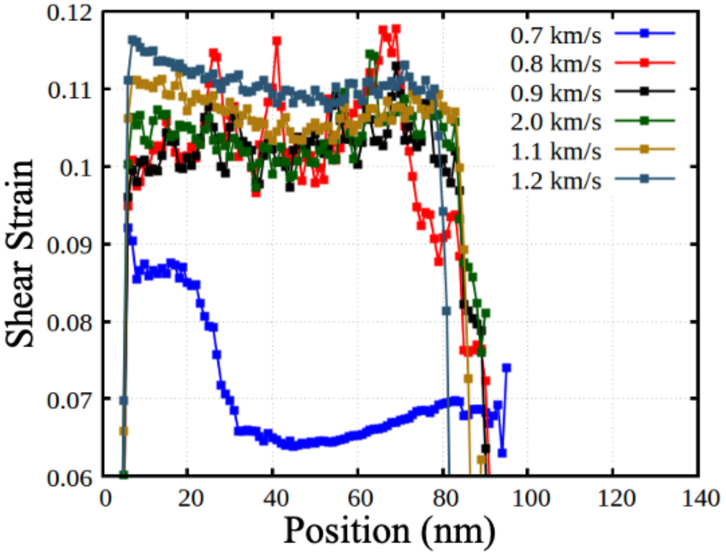

Figure S4: 1D Eulerian binning of the shear strain of all cases at 50ps held at maximum compression.

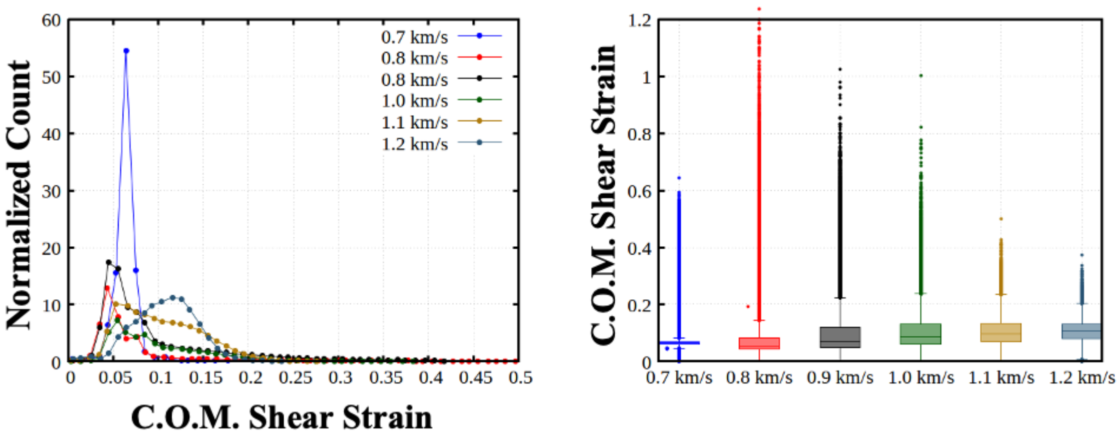

Figure S5: Distributions of molecular shear strains at 50ps held at maximum compression.

## SM-4: Lack of Phase Transition

Figure S6 shows radial distribution functions for the crystalline regions of the different shocked systems at 50ps held at maximum compression, showing the distinct lack of any phase transformation going from the shear band to non-shear band cases.

Figure S7 shows the max compression + 50ps states, colored by the $P_2[Cos(\theta)]$ metric, and a correlation plot (binned) between the $P_2[Cos(\theta)]$ and the molecular shear strain. From both plots, it is evident that the loss of molecular orientation with respect the crystal (low $P_2[Cos(\theta)]$ values) is heavily correlated with the shear strain localizations in the shear bands. For the stronger

shock cases, the loss of rotational order is more homogenous, just like the shear strain, however, the right-hand correlation plot shows very little connection between rotational changes and shearing. If a phase transformation were occurring, either a correlation would exist, or there would be a strong structure in the heat map, as molecules would rearrange into a new pattern, not rotate noisily.

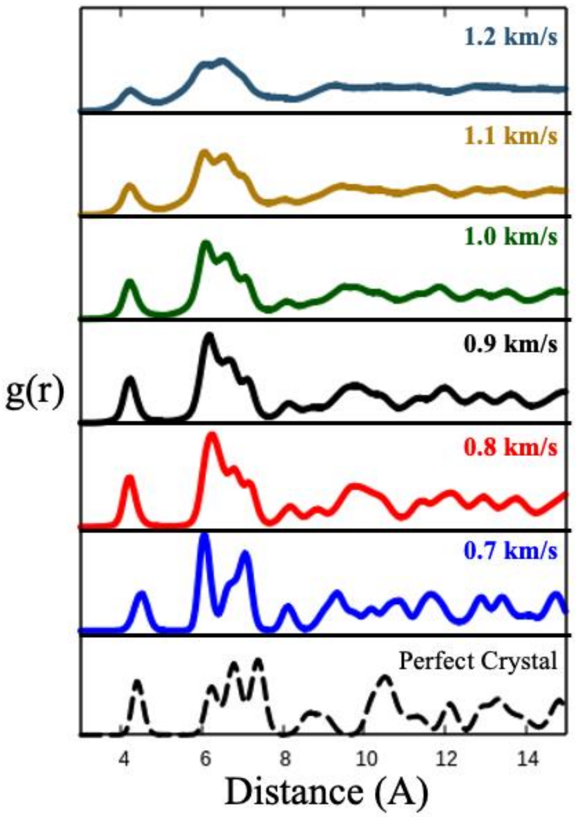


Figure S6: Radial distribution functions for the crystalline regions of the different shocked systems at 50ps held at maximum compression.

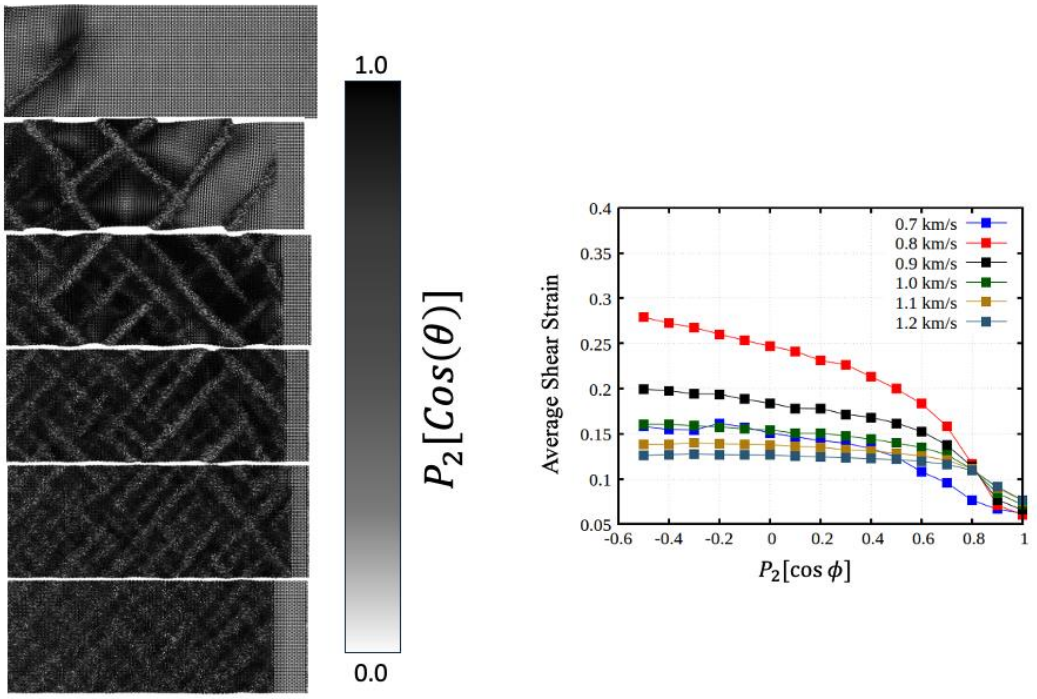


Figure S7: $P_2[Cos(\theta)]$ heat maps and correlations with shear strain for all shock strengths.

## SM-5: Release Attributes

Figure S8 shows the decay of sheared molecules during shock release such that only the non-shear band cases undergo a reversible shearing process.

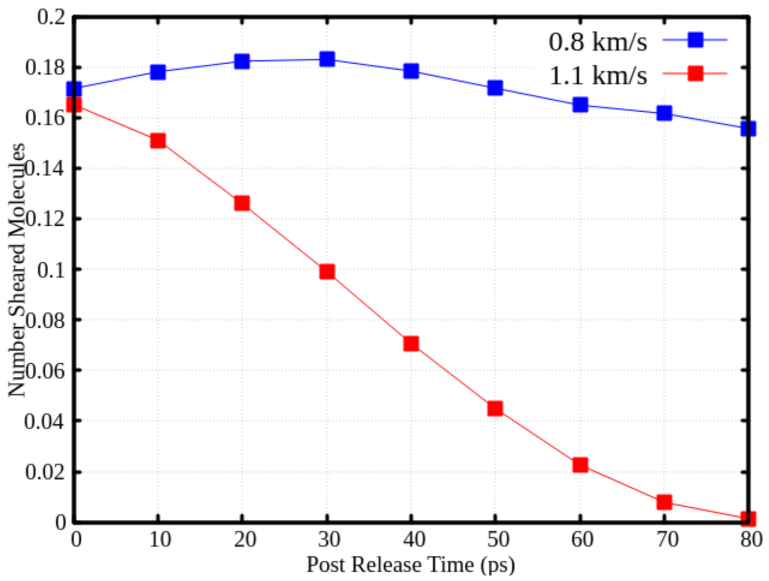

Figure S8: Number of remaining sheared molecules during release.

## SM-6: Structure of Deformation

Figure S10 shows heat maps (binned) of the Shear strain as a function of the X-Z component of the Deformation Gradient Tensor (Green-Lagrange). This shows how the movement of sheared molecules in the shear band cases (top row) follows a structure corresponding to the shear band direction and angle. However, the sheared molecules in the non-shear band cases have no structure and very little translation in the X-Z plane.

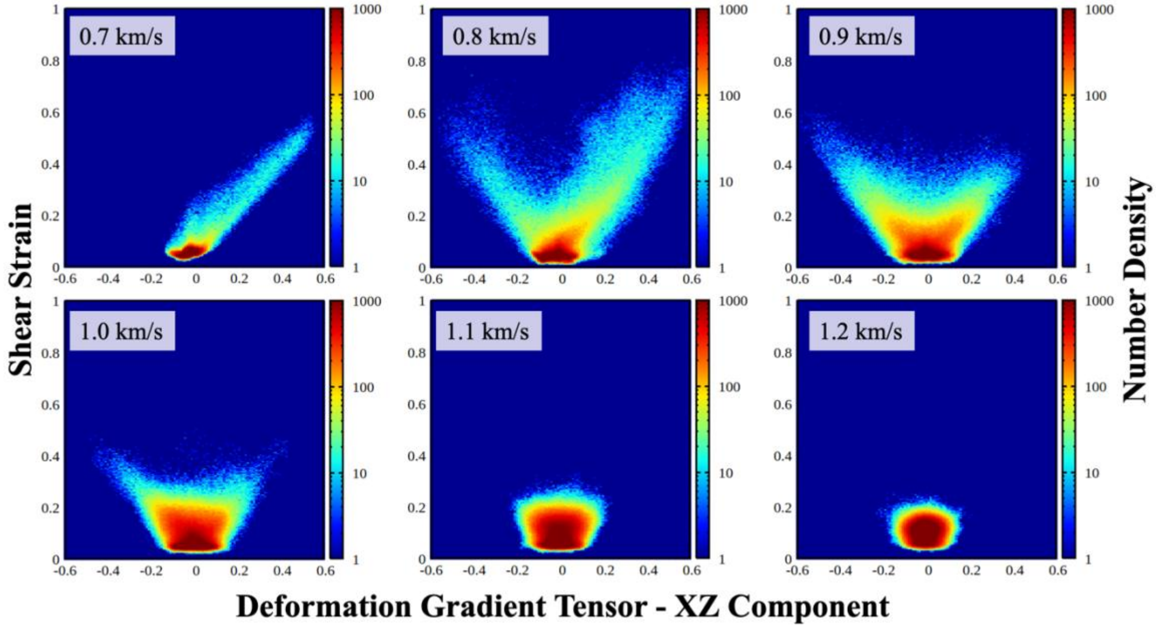

Figure S10: Heat maps (binned) of the Shear strain as a function of the X-Z component of the Deformation Gradient Tensor (Green-Lagrange).

## SM-7

Figure S11 shows molecular renderings of the sheared molecules, colored by cluster ID, showing the lack of cluster structure in the non-shear band cases.

Figure S12 shows time histories during the shock both the maximum cluster size and the number of clusters greater than 25 molecules. In the latter, the non-shear band cases have much more of these smaller cluster and, after maximum compression (19-20ps), where, in this case, release is allowed to occur immediately, there is a drastic decrease due to the shearing being a reversible mechanism. The shear band cases show no decrease in sheared molecules after release.

Figure S13 shows a composite plot of a binning of how many clusters there are of different sizes, where the point sizes reflect the total sum of molecules in those clusters.

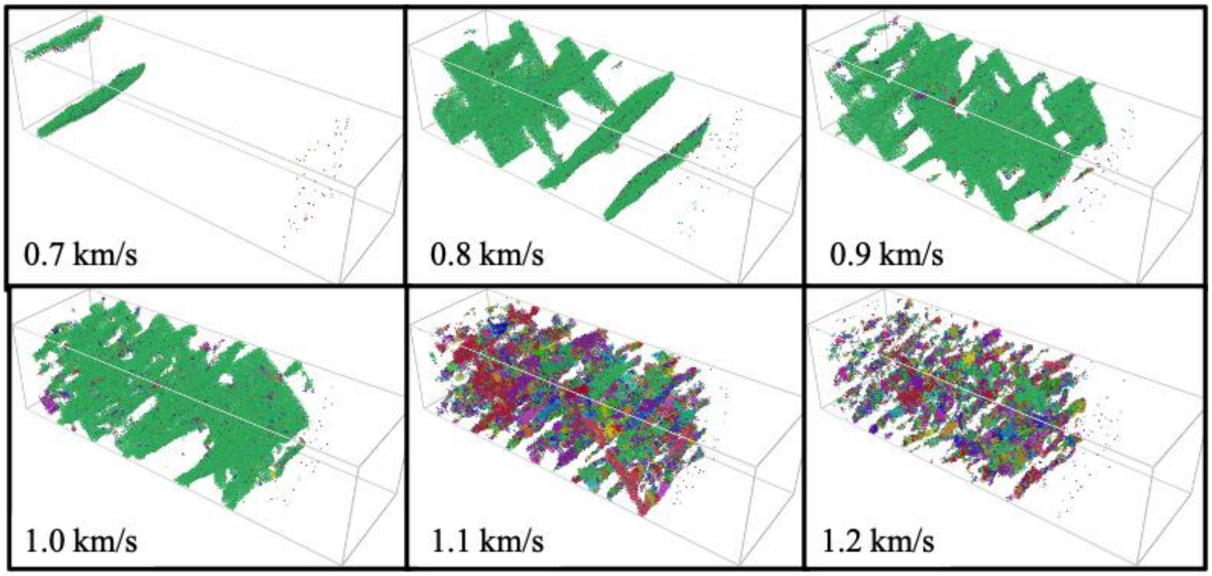


Figure S11: Molecular renderings of the sheared molecules, colored by cluster ID

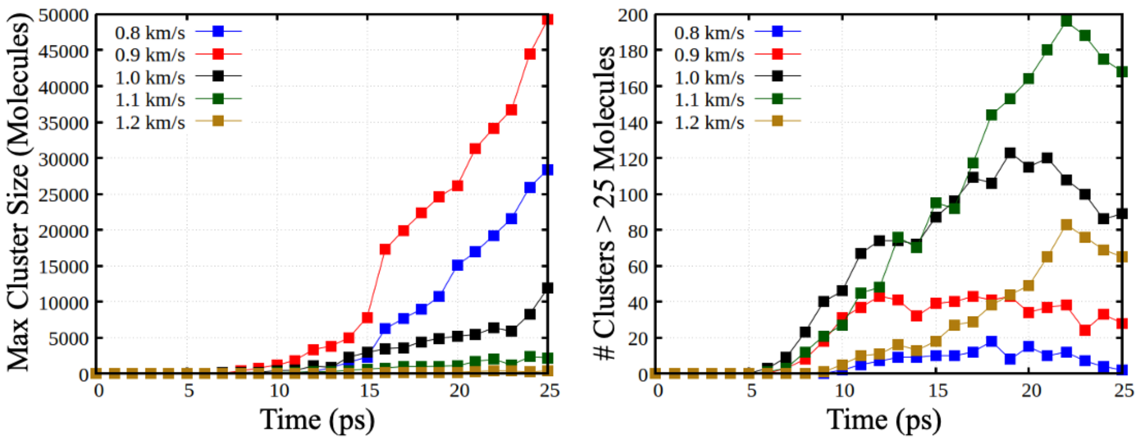


Figure S12: Time histories during the shock both the maximum cluster size and the number of clusters greater than 25 molecules.

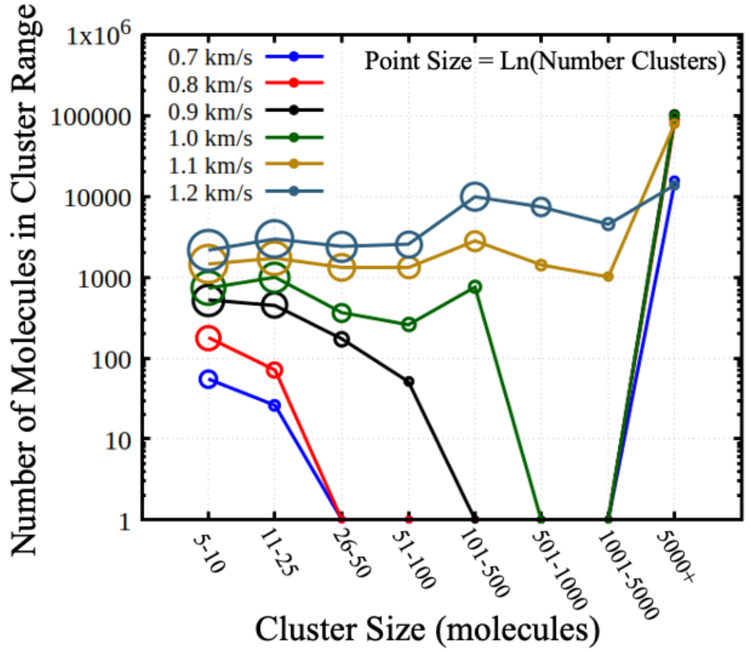


Figure S13: Composite plot of a binning of how many clusters there are of different sizes, where the point sizes reflect the total sum of molecules in those clusters.
